# Supplementary material for: Motion Without State: Probing Dynamical Consistency and Conditioning Bias in Video Models
Source: arXiv:2610.05135 source file (2026-11-24)
Supplement: Supplementary file 1 [file style_supp.tex]

\RequirePackage{tikz}
\usetikzlibrary{calc}
\RequirePackage{colortbl}
\RequirePackage{array}
\RequirePackage{tabularx}
\RequirePackage{makecell}
\RequirePackage[most]{tcolorbox}
\RequirePackage[normalem]{ulem}
\RequirePackage[T1,OT1]{fontenc}
\makeatletter
\providecommand{\degree}{\ensuremath{^\circ}}

\definecolor{sInk}{HTML}{232B3D}      %
\definecolor{sInkB}{HTML}{454D60}     %
\definecolor{sInkC}{HTML}{8A92A5}     %
\definecolor{sRule}{HTML}{CDD2DC}     %
\definecolor{sRuleB}{HTML}{9AA1B1}    %
\definecolor{sOracle}{HTML}{F3F5F8}   %
\definecolor{sFloor}{HTML}{E7ECF3}    %
\definecolor{qRespL}{HTML}{DCE9F7}\definecolor{qRespM}{HTML}{739ED4}\definecolor{qRespD}{HTML}{3F72B6}
\definecolor{qStateL}{HTML}{E1E4FA}\definecolor{qStateM}{HTML}{7381D2}\definecolor{qStateD}{HTML}{343EA5}
\definecolor{qGoalL}{HTML}{FBE3EE}\definecolor{qGoalM}{HTML}{E684AF}\definecolor{qGoalD}{HTML}{C04682}
\definecolor{qTimeL}{HTML}{FDEBDD}\definecolor{qTimeM}{HTML}{E39B73}
\definecolor{qIntL}{HTML}{EEF1F6}\definecolor{qIntM}{HTML}{8790A1}\definecolor{qIntD}{HTML}{4D566A}
\colorlet{hResp}{qRespL!72!white}
\colorlet{hState}{qStateL!72!white}
\colorlet{hGoal}{qGoalL!72!white}
\colorlet{hTime}{qTimeL!78!white}
\colorlet{hInt}{qIntL!95!white}
\colorlet{sField}{qIntL!55!white}
\colorlet{sFieldRule}{qIntM!42!white}
\definecolor{mIcecyanD}{HTML}{047C89}\definecolor{mGlacierD}{HTML}{3F72B6}\definecolor{mPeriD}{HTML}{343EA5}
\definecolor{mSlateD}{HTML}{4D566A}\definecolor{mLavD}{HTML}{724AB2}\definecolor{mOrchidD}{HTML}{812886}
\definecolor{mRoseD}{HTML}{C04682}\definecolor{mCoralD}{HTML}{AB393C}\definecolor{mPeachD}{HTML}{B0592A}

\newcommand{\supp@defmodel}[4]{%
  \@namedef{supp@mname@#1}{#2}\@namedef{supp@mshort@#1}{#3}\@namedef{supp@mfile@#1}{#4}}
\supp@defmodel{ltx23}{LTX-2.3}{LTX-2.3}{ltx23_full}
\supp@defmodel{ltx25d}{LTX-2.5 (distilled)}{LTX-2.5 dist.}{ltx25_distilled}
\supp@defmodel{ltx25}{LTX-2.5}{LTX-2.5}{ltx25_full}
\supp@defmodel{cosmos}{Cosmos 3 Nano}{Cosmos 3 Nano}{cosmos3_nano}
\supp@defmodel{h3}{MiniMax-H3}{MiniMax-H3}{minimax_h3}
\supp@defmodel{wan22}{Wan 2.2 (A14B)}{Wan 2.2}{wan22_i2v_a14b}
\supp@defmodel{wan30}{Wan 3.0}{Wan 3.0}{wan30}
\supp@defmodel{sd20}{Seedance 2.0}{Seedance 2.0}{seedance20}
\supp@defmodel{sd20mini}{Seedance 2.0 mini}{Seedance mini}{seedance20_mini}
\supp@defmodel{tiv5b}{Wan 2.2 (TI2V-5B)}{Wan 2.2 5B}{}
\newcommand{\supp@glyphfile}[1]{\raisebox{-0.14ex}{\includegraphics[height=0.72em]{figs/glyphs/#1.pdf}}}
\DeclareRobustCommand{\mglyph}[1]{%
  \edef\supp@file{\@nameuse{supp@mfile@#1}}%
  \ifx\supp@file\@empty
    \tikz[baseline=-0.55ex]{\draw[mSlateD,line width=0.5pt] (-0.6mm,-0.6mm)--(0.6mm,0.6mm) (-0.6mm,0.6mm)--(0.6mm,-0.6mm);}%
  \else
    \supp@glyphfile{\supp@file}%
  \fi}
\DeclareRobustCommand{\mname}[1]{\makebox[2.6mm][c]{\mglyph{#1}}\,\@nameuse{supp@mname@#1}}
\DeclareRobustCommand{\mshort}[1]{\makebox[2.6mm][c]{\mglyph{#1}}\,\@nameuse{supp@mshort@#1}}

\newcommand{\supphdrcolor}{hInt}
\newenvironment{stab}[2]{%
  \renewcommand{\supphdrcolor}{#1}%
  \setlength{\aboverulesep}{0pt}\setlength{\belowrulesep}{0pt}%
  \setlength{\extrarowheight}{0.9pt}%
  \renewcommand{\arraystretch}{1.18}%
  \arrayrulecolor{sInk}%
  \begin{tabular}{#2}}{\end{tabular}}
\newcommand{\shead}{\rowcolor{\supphdrcolor}}
\newcommand{\bandrule}{\arrayrulecolor{sInkB}\specialrule{0.4pt}{0pt}{0pt}\arrayrulecolor{sInk}}
\newcommand{\oraclelabel}{\makebox[2.6mm][c]{\supp@glyphfile{physics}}\,Physical oracle}
\newcommand{\oraclerow}{\rowcolor{sOracle}}
\newcommand{\oraclerule}{\arrayrulecolor{sRuleB}\specialrule{0.5pt}{0pt}{0pt}\arrayrulecolor{sInk}}
\newcommand{\grouprule}{\arrayrulecolor{sRule}\specialrule{0.35pt}{0.6pt}{0.6pt}\arrayrulecolor{sInk}}
\newcommand{\rowrule}{\arrayrulecolor{sRule}\specialrule{0.25pt}{0pt}{0pt}\arrayrulecolor{sInk}}
\newcommand{\hu}[1]{{\color{sInkC}#1}}
\def\snum#1{\supp@snum#1\relax\@nil}
\def\supp@snum#1#2\@nil{\ifx-#1\textminus\supp@strip#2\else#1\supp@strip#2\fi}
\def\supp@strip#1\relax{#1}
\newcommand{\ci}[2]{{\leavevmode\color{sInkC}\tiny[\snum{#1},\,\snum{#2}]}}
\newcommand{\nn}[1]{{\leavevmode\color{sInkC}\tiny(#1)}}
\newcommand{\gnote}[1]{{\leavevmode\color{sInkC}#1}}
\newcommand{\nd}{{\leavevmode\color{sInkC}\textendash}}
\newcommand{\vci}[3]{\makecell[c]{\snum{#1}\\[-2.4pt]\ci{#2}{#3}}}
\newcommand{\vcin}[4]{\makecell[c]{\snum{#1}\\[-2.4pt]\ci{#2}{#3}\,\nn{#4}}}
\newcommand{\perarm}[2]{\includegraphics[width=\linewidth,trim=0 #2 0 #1,clip]{figs/supp_perarm.pdf}}
\newcommand{\perarmhead}{\perarm{0}{581.3}}

\newlength{\ivw}\setlength{\ivw}{13mm}
\newcommand{\supp@bandlo}{}\newcommand{\supp@bandhi}{}
\newcommand{\ivband}[2]{\def\supp@bandlo{#1}\def\supp@bandhi{#2}}
\newcommand{\ivbar}[7][sInk]{%
  \begin{tikzpicture}[baseline=-0.6ex,x=\ivw/(#7-#6)]
    \useasboundingbox (#6,-0.9mm) rectangle (#7,0.9mm);
    \ifx\supp@bandlo\@empty\else
      \fill[sFloor] (\supp@bandlo,-0.75mm) rectangle (\supp@bandhi,0.75mm);
    \fi
    \draw[sRule,line width=0.3pt] (#6,0)--(#7,0);
    \draw[sInk,line width=0.55pt] (#5,-0.85mm)--(#5,0.85mm);
    \pgfmathsetmacro{\supp@lo}{max(#2,#6)}\pgfmathsetmacro{\supp@hi}{min(#4,#7)}
    \draw[#1,line width=0.85pt,line cap=round] (\supp@lo,0)--(\supp@hi,0);
    \pgfmathsetmacro{\supp@v}{min(max(#3,#6),#7)}
    \fill[white] (\supp@v,0) circle (0.62mm);
    \fill[#1] (\supp@v,0) circle (0.48mm);
  \end{tikzpicture}\gdef\supp@bandlo{}\gdef\supp@bandhi{}}
\newcommand{\rangebar}[5]{%
  \begin{tikzpicture}[baseline=-0.6ex,x=\ivw/(#5-#4)]
    \useasboundingbox (#4,-0.9mm) rectangle (#5,0.9mm);
    \draw[sRule,line width=0.3pt] (#4,0)--(#5,0);
    \fill[qIntM!55] (#1,-0.55mm) rectangle (#2,0.55mm);
    \draw[sInk,line width=0.6pt] (#3,-0.85mm)--(#3,0.85mm);
  \end{tikzpicture}}
\newlength{\shw}\setlength{\shw}{10mm}
\newcommand{\sharebar}[3]{%
  \begin{tikzpicture}[baseline=-0.6ex]
    \fill[qIntL] (0,-0.62mm) rectangle (\shw,0.62mm);
    \pgfmathsetmacro{\supp@r}{#2/#3}\pgfmathsetmacro{\supp@i}{#1/#3}
    \fill[qIntM] (0,-0.62mm) rectangle ({\supp@r*\shw},0.62mm);
    \fill[qIntD] (0,-0.62mm) rectangle ({\supp@i*\shw},0.62mm);
    \draw[qIntM,line width=0.25pt] (0,-0.62mm) rectangle (\shw,0.62mm);
  \end{tikzpicture}}
\newlength{\dbw}\setlength{\dbw}{13mm}
\newcommand{\dumbbell}[4][qGoalD]{%
  \begin{tikzpicture}[baseline=-0.6ex,x=\dbw/100]
    \useasboundingbox (0,-0.9mm) rectangle (100,0.9mm);
    \ifx\supp@bandlo\@empty\else
      \fill[sFloor] (\supp@bandlo,-0.75mm) rectangle (\supp@bandhi,0.75mm);
    \fi
    \draw[sRule,line width=0.3pt] (0,0)--(100,0);
    \if\relax\detokenize{#4}\relax\else\draw[sInk,line width=0.55pt] (#4,-0.85mm)--(#4,0.85mm);\fi
    \draw[#1,line width=0.7pt] (#2,0)--(#3,0);
    \fill[#1] (#2,0) circle (0.55mm);
    \fill[white] (#3,0) circle (0.5mm);\draw[#1,line width=0.45pt] (#3,0) circle (0.5mm);
  \end{tikzpicture}\gdef\supp@bandlo{}\gdef\supp@bandhi{}}
\newcommand{\tribar}[6]{%
  \begin{tikzpicture}[baseline=-0.6ex]
    \pgfmathsetmacro{\supp@t}{max(#1+#2+#3,1)}
    \pgfmathsetmacro{\supp@a}{#1/\supp@t}\pgfmathsetmacro{\supp@b}{(#1+#2)/\supp@t}
    \fill[#6] (0,-0.62mm) rectangle (\shw,0.62mm);
    \fill[#5] (0,-0.62mm) rectangle ({\supp@b*\shw},0.62mm);
    \fill[#4] (0,-0.62mm) rectangle ({\supp@a*\shw},0.62mm);
    \draw[qIntM,line width=0.25pt] (0,-0.62mm) rectangle (\shw,0.62mm);
  \end{tikzpicture}}
\newcommand{\fracbar}[3][qIntD]{%
  \begin{tikzpicture}[baseline=-0.6ex]
    \fill[qIntL] (0,-0.62mm) rectangle (\shw,0.62mm);
    \pgfmathsetmacro{\supp@r}{#2/#3}
    \fill[#1] (0,-0.62mm) rectangle ({\supp@r*\shw},0.62mm);
    \draw[qIntM,line width=0.25pt] (0,-0.62mm) rectangle (\shw,0.62mm);
  \end{tikzpicture}}
\newcommand{\spark}[4]{%
  \begin{tikzpicture}[baseline={([yshift=-0.75ex]current bounding box.center)},x=3.9mm,y=2.8mm/(#3-#2)]
    \useasboundingbox ($(-0.2,#2)+(0,-0.5pt)$) rectangle ($(3.2,#3)+(0,0.5pt)$);
    \fill[qIntL!60] (-0.12,#2) rectangle (3.12,#3);
    \draw[sInk,line width=0.45pt,dash pattern=on 1.1pt off 0.7pt] (-0.12,#4)--(3.12,#4);
    \foreach \v [count=\i from 0, remember=\v as \u] in {#1} {\ifnum\i>0 \draw[qRespD,line width=0.6pt] (\i-1,\u)--(\i,\v);\fi}
    \foreach \v [count=\i from 0] in {#1} {\fill[qRespD] (\i,\v) circle (0.3mm);}
  \end{tikzpicture}}
\newcommand{\lenspark}[4][sInk]{%
  \begin{tikzpicture}[baseline={([yshift=-0.75ex]current bounding box.center)},x=1.25mm,y=2.8mm/(#4-#3)]
    \useasboundingbox ($(-0.4,#3)+(0,-0.5pt)$) rectangle ($(5.4,#4)+(0,0.5pt)$);
    \fill[qIntL!60] (-0.3,#3) rectangle (5.3,#4);
    \foreach \v [count=\i] in {#2} {\ifcase\i\or\xdef\supp@pa{(0,\v)}\or\xdef\supp@pb{(2,\v)}\or\xdef\supp@pc{(5,\v)}\fi}
    \draw[#1,line width=0.6pt] \supp@pa--\supp@pb--\supp@pc;
    \foreach \p in {\supp@pa,\supp@pb,\supp@pc} {\fill[#1] \p circle (0.3mm);}
  \end{tikzpicture}}
\newcommand{\outbar}[4]{%
  \begin{tikzpicture}[baseline=-0.6ex,x=1.25mm]
    \pgfmathtruncatemacro{\supp@a}{#1}\pgfmathtruncatemacro{\supp@b}{#1+#2}\pgfmathtruncatemacro{\supp@c}{#1+#2+#3}\pgfmathtruncatemacro{\supp@d}{#1+#2+#3+#4}
    \useasboundingbox (0,-0.8mm) rectangle (\supp@d,0.8mm);
    \foreach \i in {1,...,\supp@d}{%
      \ifnum\i>\supp@c \def\supp@col{qGoalM}\else\ifnum\i>\supp@b \def\supp@col{qIntM}\else\ifnum\i>\supp@a \def\supp@col{qStateM}\else\def\supp@col{qStateD}\fi\fi\fi
      \fill[\supp@col] (\i-1+0.12,-0.62mm) rectangle (\i-0.12,0.62mm);}
  \end{tikzpicture}}
\DeclareRobustCommand{\okey}[2]{\tikz[baseline=-0.6ex]\fill[#1] (0,-0.62mm) rectangle (1mm,0.62mm);\,#2}
\DeclareRobustCommand{\okeyf}[2]{\tikz[baseline=-0.6ex]\filldraw[fill=#1,draw=qIntM,line width=0.25pt] (0,-0.62mm) rectangle (1mm,0.62mm);\,#2}
\newcommand{\pips}[2]{%
  \begin{tikzpicture}[baseline=-0.6ex,x=1.25mm]
    \useasboundingbox (0,-0.7mm) rectangle (#2,0.7mm);
    \foreach \i in {1,...,#2}{%
      \ifnum\i>#1 \draw[qStateD,line width=0.35pt] (\i-0.5,0) circle (0.42mm);\else\fill[qStateD] (\i-0.5,0) circle (0.48mm);\fi}
  \end{tikzpicture}}
\newcommand{\tilebox}[4]{%
  \tikz[baseline=(spt.base)]{%
    \node[inner xsep=1.7pt,inner ysep=#3,outer sep=0pt,minimum width=#2,fill=#1,rounded corners=1.3pt] (spt) {#4};
    \path ([yshift=1.3pt]spt.north) ([yshift=-1.3pt]spt.south);}}
\newcommand{\tile}[2][qRespL]{\tilebox{#1}{0pt}{1.1pt}{#2}}
\newcommand{\tilec}[2][qRespL]{\tilebox{#1}{0pt}{0pt}{#2}}
\newcommand{\tilew}[3]{\tilebox{#1}{#2}{0pt}{#3}}
\newcommand{\heattile}[5]{%
  \pgfmathtruncatemacro{\supp@p}{min(abs(#2)/#3,1)*46}%
  \edef\supp@tmp{\noexpand\tilebox{#1!\supp@p!white}{#4}{0pt}}\supp@tmp{#5}}
\newlength{\supp@gclear}\setlength{\supp@gclear}{1.6pt}
\newcommand{\gpad}[1]{\raisebox{0pt}[\dimexpr\height+\supp@gclear\relax][\dimexpr\depth+\supp@gclear\relax]{#1}}
\DeclareRobustCommand{\notrun}[1][10mm]{%
  \begin{tikzpicture}[baseline=-0.62ex]
    \pgfmathsetlengthmacro{\supp@w}{#1/2}
    \pgfmathsetlengthmacro{\supp@h}{1.3mm}
    \useasboundingbox (-\supp@w-0.2mm,-\supp@h-0.2mm) rectangle (\supp@w+0.2mm,\supp@h+0.2mm);
    \begin{scope}
      \clip (-\supp@w,-\supp@h) rectangle (\supp@w,\supp@h) (-3.45mm,1.02mm) rectangle (3.45mm,-0.98mm);
      \foreach \k in {-16,...,16}{%
        \draw[sInkC!85,line width=0.27pt,line cap=round] (\k*0.74mm-1.3mm,-1.3mm)--++(2.6mm,2.6mm);}
    \end{scope}
    \draw[sInkC,line width=0.45pt,line cap=round]
      (-\supp@w-0.16mm,-\supp@h+0.05mm) .. controls (-0.3*\supp@w,-\supp@h-0.13mm) and (0.4*\supp@w,-\supp@h+0.11mm) .. (\supp@w+0.12mm,-\supp@h-0.03mm)
      (\supp@w+0.03mm,-\supp@h-0.17mm) .. controls (\supp@w+0.11mm,-0.3*\supp@h) and (\supp@w-0.09mm,0.4*\supp@h) .. (\supp@w-0.02mm,\supp@h+0.13mm)
      (\supp@w+0.14mm,\supp@h-0.02mm) .. controls (0.35*\supp@w,\supp@h+0.12mm) and (-0.45*\supp@w,\supp@h-0.09mm) .. (-\supp@w-0.09mm,\supp@h+0.04mm)
      (-\supp@w+0.02mm,\supp@h+0.14mm) .. controls (-\supp@w-0.11mm,0.3*\supp@h) and (-\supp@w+0.08mm,-0.35*\supp@h) .. (-\supp@w-0.03mm,-\supp@h-0.13mm);
    \node[inner sep=0pt,text=sInkB,font=\fontsize{5.2}{5.2}\selectfont\itshape] at (0,0.02mm) {not run};
  \end{tikzpicture}}
\DeclareRobustCommand{\okmark}{\tikz[baseline=-0.6ex]\draw[qRespD,line width=0.7pt,line cap=round,line join=round] (-0.75mm,0)--(-0.2mm,-0.55mm)--(0.85mm,0.65mm);}
\DeclareRobustCommand{\flagmark}{\tikz[baseline=-0.6ex]\draw[qGoalD,line width=0.7pt,line cap=round] (-0.6mm,-0.6mm)--(0.6mm,0.6mm) (-0.6mm,0.6mm)--(0.6mm,-0.6mm);}
\newcommand{\supplist}[1]{\foreach \x [count=\i] in {#1}{\ifnum\i>1, \fi\x}}
\newcommand{\readcard}[6]{%
  \begin{tcolorbox}[enhanced,colback=white,colframe=sRule,boxrule=0.3pt,arc=1mm,left=1.3mm,right=1.3mm,top=0.8mm,bottom=0.9mm,
    fontupper=\scriptsize,colbacktitle=#1,coltitle=sInk,fonttitle=\scriptsize,titlerule=0pt,toptitle=0.4mm,bottomtitle=0.4mm,
    lefttitle=1.3mm,title={{\small #2}\hspace{0.6em}#3}]
    \raggedright #4\par\vspace{1.2pt}{\color{sRule}\hrule height 0.25pt}\vspace{1.4pt}
    {\color{sInkC}oracle}\hspace{0.4em}#5\par
    {\color{sInkC}floor}\hspace{0.4em}#6
  \end{tcolorbox}}

\tcbset{
  supp card/.style={enhanced,breakable,colback=white,colframe=sRule,boxrule=0.4pt,arc=1.2mm,
    left=1.6mm,right=1.6mm,top=1.2mm,bottom=1.4mm,before skip=5pt,after skip=7pt,fontupper=\footnotesize,
    fonttitle=\small,coltitle=sInk,colbacktitle=white,toptitle=0.6mm,bottomtitle=0.3mm,
    titlerule=0pt,attach boxed title to top left={xshift=2mm,yshift*=-\tcboxedtitleheight/2},
    boxed title style={colback=white,colframe=white,boxrule=0pt,arc=0.6mm,left=0.8mm,right=0.8mm,top=0pt,bottom=0pt}},
}
\let\supp@tcb@split@USL\tcb@split@USL
\def\tcb@split@USL{%
  \tcb@comp@h@page
  \ifdim\tcb@h@page<18mm\relax\null\pagebreak\fi
  \supp@tcb@split@USL}
\newcommand{\cardtag}[2]{{\setlength{\fboxsep}{0.8pt}\colorbox{#1}{\scriptsize\color{sInkB}\,#2\,}}}
\newcommand{\suppneed}[1]{\par\begingroup\setlength{\dimen@}{#1\baselineskip}%
  \vskip\z@\@plus\dimen@\penalty-100\vskip\z@\@plus-\dimen@\vskip\dimen@\penalty9999\vskip-\dimen@\vskip\z@skip\endgroup}
\newcommand{\cardsep}{\par\penalty-50\vskip2pt
  \cleaders\hbox to\linewidth{{\color{sRule}\vrule width\linewidth height 0.3pt depth 0pt}}\vskip0.3pt
  \vskip3pt\relax}
\newenvironment{scardp}[3][qIntL]{%
  \begin{tcolorbox}[supp card,lines before break=7,title={\textbf{#2}\hspace{0.6em}\cardtag{#1}{#3}}]\captionsetup{font=scriptsize,skip=2pt,hypcap=false}}{\end{tcolorbox}}
\newenvironment{scard}[3][qIntL]{%
  \begin{tcolorbox}[supp card,title={\textbf{#2}\hspace{0.6em}\cardtag{#1}{#3}}]\captionsetup{font=scriptsize,skip=2pt,hypcap=false}}{\end{tcolorbox}}
\newlength{\supp@elabelw}\setlength{\supp@elabelw}{13mm}
\newdimen\supp@sh\newdimen\supp@sd
\newsavebox{\supp@etext}\newsavebox{\supp@eout}\newsavebox{\supp@eline}
\newbox\supp@pbox
\newif\ifsupp@efirst
\newcommand{\supp@elabel}{}
\def\supp@emit#1#2{%
  \setbox\supp@eline=\hbox{#1}%
  \supp@sh=\ht\supp@eline \ifdim\supp@sh<6.9pt \supp@sh=6.9pt\fi
  \supp@sd=\dp\supp@eline \ifdim\supp@sd<2.6pt \supp@sd=2.6pt\fi
  \ifsupp@efirst\else\ifnum#2<10000 \penalty50 \fi\fi
  \nointerlineskip
  \hbox to\linewidth{\rlap{\color{sField}\vrule width\linewidth height\supp@sh depth\supp@sd}%
    \hskip2.3mm\ifsupp@efirst\hbox to\supp@elabelw{\color{sInkB}\scriptsize\supp@elabel\hss}\else\hskip\supp@elabelw\fi
    \hskip1.2mm\box\supp@eline\hss}%
  \global\supp@efirstfalse}
\def\supp@peel{\setbox\supp@pbox=\lastbox
  \ifvoid\supp@pbox\else
    \unskip\count@=\lastpenalty\unpenalty\unskip\unpenalty
    \edef\supp@thispen{\the\count@}%
    {\supp@peel}\supp@emit{\box\supp@pbox}{\supp@thispen}\fi}
\newcommand{\supp@entrybody}[2]{%
  \def\supp@elabel{#1}%
  \setbox\supp@etext=\vbox{\hsize=\dimexpr\linewidth-4.6mm-\supp@elabelw-1.2mm\relax
    \clubpenalty=10000 \widowpenalty=10000 \interlinepenalty=0
    \footnotesize\raggedright\noindent #2\par}%
  \global\supp@efirsttrue
  \setbox\supp@eout=\vbox{\unvbox\supp@etext\supp@peel}%
  \unvbox\supp@eout}
\newcommand{\supp@estrip}[1]{%
  \nointerlineskip
  \hbox to\linewidth{\tikz{\useasboundingbox (0,0) rectangle (\linewidth,1.9mm);
    \clip (0,0) rectangle (\linewidth,1.9mm);
    \if t#1\fill[sField,rounded corners=0.8mm] (0,-1.5mm) rectangle (\linewidth,1.9mm);%
    \else\fill[sField,rounded corners=0.8mm] (0,0) rectangle (\linewidth,3.4mm);\fi}\hss}}
\newcommand{\supp@fsep}{%
  \par\nointerlineskip\penalty-50
  \cleaders\hbox to\linewidth{%
    \rlap{\color{sField}\vrule width\linewidth height 4.4pt depth 0pt}%
    \hskip 2.3mm\raise2.05pt\hbox{\color{sFieldRule}\vrule width\dimexpr\linewidth-4.6mm\relax height 0.3pt depth 0pt}%
    \hss}\vskip 4.4pt\relax}
\newcommand{\fentry}[3]{%
  \if f#1\par\vspace{3pt}\supp@estrip{t}\nobreak\fi\if s#1\par\vspace{3pt}\supp@estrip{t}\nobreak\fi
  \if m#1\supp@fsep\fi\if l#1\supp@fsep\fi
  \supp@entrybody{#2}{#3}%
  \if l#1\nobreak\supp@estrip{b}\par\vspace{1pt}\fi\if s#1\nobreak\supp@estrip{b}\par\vspace{1pt}\fi}
\newcommand{\fields}[4]{%
  \fentry{f}{held fixed}{#1}\fentry{m}{changed}{#2}\fentry{m}{law predicts}{#3}\fentry{l}{isolates}{#4}}
\DeclareRobustCommand{\cbox}[1]{\tikz[baseline=-0.62ex]{\draw[sInkB,line width=0.35pt,rounded corners=0.2mm] (-0.72mm,-0.72mm) rectangle (0.72mm,0.72mm);
  \ifnum#1=1 \draw[qRespD,line width=0.62pt,line cap=round,line join=round] (-0.48mm,0.02mm)--(-0.1mm,-0.4mm)--(0.62mm,0.58mm);\fi}}
\newcommand{\prompttt}{\fontencoding{T1}\fontfamily{zi4}\selectfont}
\newcommand{\slot}[1]{{\setlength{\fboxsep}{0.5pt}\colorbox{qGoalL}{\strut\{#1\}}}}
\newenvironment{promptcard}[2]{\begin{tcolorbox}[supp card,unbreakable,fonttitle=\footnotesize,title={\textbf{#1}\hspace{0.5em}\cardtag{hInt}{#2}}]}{\end{tcolorbox}}
\newcommand{\pfields}[2]{%
  \begin{tabularx}{\linewidth}{@{}>{\raggedright\arraybackslash\leavevmode\color{sInkB}\scriptsize}p{11.5mm}@{\hspace{1.2mm}}>{\raggedright\arraybackslash\scriptsize}X@{}}
    used in & #1\\[1pt]
    names the outcome & #2
  \end{tabularx}}
\newcommand{\ptext}[1]{%
  \begin{tcolorbox}[enhanced,colback=sField,colframe=sField,boxrule=0pt,arc=0.8mm,left=1.4mm,right=1.4mm,
    top=1mm,bottom=1mm,before skip=2.5pt,after skip=0pt,fontupper=\prompttt\scriptsize\raggedright]#1\end{tcolorbox}}
\newcommand{\cbl}[2]{\mbox{\cbox{#1}\,#2}\hspace{0.9em}}
\newcommand{\thumb}[2][\linewidth]{\begingroup\setlength{\fboxsep}{0pt}\setlength{\fboxrule}{0.3pt}\color{sRule}%
  \fbox{\includegraphics[width=\dimexpr#1-0.6pt\relax]{#2}}\endgroup}
\newcommand{\thumbcap}[1]{{\color{sInkC}\scriptsize #1}}
\makeatother
